# Supplementary material for: BoostMIS: Boosting Medical Image Semi-supervised Learning with Adaptive Pseudo Labeling and Informative Active Annotation
Source: arXiv:2203.02533 source file (2022-03-21)
Supplement: Supplementary file 1 [file appendix.tex]

% CVPR 2022 Paper Template
% based on the CVPR template provided by Ming-Ming Cheng (https://github.com/MCG-NKU/CVPR_Template)
% modified and extended by Stefan Roth (stefan.roth@NOSPAMtu-darmstadt.de)

%%%%%%%%% PAPER ID  - PLEASE UPDATE
 % *** Enter the CVPR Paper ID here

%%%%%%%%% TITLE - PLEASE UPDATE

\newpage
\newpage
This appendix provides the implementation details (Section~\ref{sec:ID}), MESCC dataset details (Section~\ref{sec:MD}) and more experimental results on MESCC dataset (Section~\ref{sec:exp_MESCC}). It also reports the additional experimental results on COVIDx dataset~\cite{wang2020covid} (Seciton~\ref{sec:exp_COVID}). Finally, we list the limitations and societal impact of this paper (Section~\ref{sec:LSI}).

% For instance, pseudo-labeling produces pseudo-labels for unlabeled data via model's class prediction, and then train the model against to improve the performance.
%%%%%%%%% ABSTRACT

\section{Implementation Details}\label{sec:ID}
\noindent\textbf{Training Details.} In the medical image classification under semi-supervised learning (SSL), we adopt FixMatch~\cite{berthelot2019mixmatch} as our SSL method, where Wide ResNet-50~\cite{he2016deep} is the backbone of the task model. To train the AL-based SSL model with a balanced initialization, we set up the initial labeled pool (10\% data) by uniformly sampling in each class. The initial labeled pool is a subset of the training set (30\% data) for pure SSL models, and other SSL training data are randomly sampled. We follow~\cite{gao2020consistency} for the AL budget that determines the selected capacity. In Section 3.5, the hyperparameter $M$ is set to 20 to estimate the cosine similarity between the unselected sample $u^u_i$ and its nearest samples in the distribution space.
From our empirical experiments, the unsupervised loss hyperparameter $\mu$ is defined as 1. We train the \method{} with standard stochastic gradient descent (SGD)~\cite{bottou2010large} optimizer with an initial learning rate of 0.03, a momentum of 0.9 and weight decay of 0.0005 in all experiments.  Batch size and total training step are set to 64 and 100,000, respectively. The coefficients $\alpha$ and $\beta$ of the adaptive threshold are defined as 0.9 and 0.05, respectively. When the iterative training step is over 5,0000, the high confidence threshold will be set to 0.95. The loss function for \method{} consists of two cross-entropy loss terms: a supervised loss $\ell_s(\theta_{\mathcal{S}})$ applied to labeled data and an unsupervised loss $\ell_u(\theta_{\mathcal{S}})$. Thus the full objective function is:
\begin{equation}
     \ell(\theta_{\mathcal{S}}) =   \ell_s(\theta_{\mathcal{S}})+ \ell_s(\theta_{\mathcal{S}}) 
\end{equation}

\noindent\textbf{Experimental Environment.} The experiments are conducted on a server with Xeon(R) Silver 4114 CPU @ 2.2GHz (10 cores), 256G memory and GeForce RTX 2080 Ti (8 GPUs). Models are implemented in PyTorch 1.6.0 with CUDA 10.2.

  % Use Input in the format of Algorithm
% \renewcommand{\algorithmicensure}{\textbf{Output:}} % Use Output in the format of Algorithm

\begin{algorithm}[t]
  \caption{\method{}: Boosting Medical Image Semi-supervised Learning  Framework}
   \textbf{Input}:Paired  samples ($\mathcal{X}$, $\mathcal{Y}$) with supervised information, unlabeled samples  $\mathcal{U}$; \\
   \textbf{Initialization}: Construct initial labeled pool $IP$= 10\% labeled data, define the AL cycles $AC$= 30;\\
  \Repeat{Convergence}{ \If{ SSL model in \method{} have not trained}
        {
          \Repeat { Convergence}{
           Randomly sample a minibatch;\\
           Train task model $T(\cdot;\theta_S)$ with paired ($\mathcal{X}$, $\mathcal{Y}$) using Eqn.(2); \\
           \If{Training step $\leq$ 50,000 }
           {
                Set adaptive threshold  $\epsilon_{t}$ $\Longleftarrow$ ($\alpha$, 
                $\beta$, $N_A$, $K$, $Count_{\epsilon_{t-1}}$, $Count_{\epsilon_{t}}$) using Eqn.(3);\\
           }
            \Else{Set adaptive threshold $\epsilon_{t}$ $\Longleftarrow$ $\alpha$+$\beta$;}\\
            Propagate label information from ($\mathcal{X}$, $\mathcal{Y}$) to unlabeled sample $\mathcal{U}^s$ ;\\
           Update $\theta_{\mathcal{S}}$ using Eqn.(5);\\
           }
        }
            Compute \textbf{r}^{adv} $\Longleftarrow$ ($\tau$, $\textbf{r}^u$, $\Delta r$) using Eqn.(7);\\
            Select top-$K$ unstable samples with largest variance from  $\mathcal{U}^u$ using Eqn.(8);\\
            Select top-$K$ uncertain samples with largest entropy from  $\mathcal{U}^u$ using Eqn.(9), (10);\\
            Update labeled pool $IP$ = $IP$ \cup $N_A$ ($N_A$$\leq$$2K$);\\
        }
 \Return{Task model $T(\cdot;\theta_S)$  trained with ($\mathcal{X}$, $\mathcal{Y}$, $\mathcal{U}$) }.
\label{alg}
\end{algorithm}

\noindent\textbf{Algorithm.} 
As presented in the main text, SSL and AL algorithms have been designed to work collaboratively to achieve better medical image SSL in our proposed framework. Algorithm 1 presents the pseudocode of our \method{}: (1) On the one hand, the label propagator can propagate the supervised label information to unlabeled samples by adaptive pseudo-labeling and augmentation-aware consistency regularization. This training strategy can mix up the pseudo-labeled samples that provide extra explicit training signals and initial labeled samples to improve the task model's performance. (2) On the other hand, the adversarial unstability selector and the balanced uncertainty selector let the oracle annotate the samples with the largest inconsistency and the highest uncertainty, which could assist the SSL model in including the informative samples for better label propagation. In summary, the proposed \method{} lets SSL and AL models work collaboratively and form a closed-loop naturally to boost the medical image SSL.

\begin{table}[t]
\small
\caption{ \textbf{Patient demographics and clinical characteristics for the MESCC dataset.}}
\centering
\begin{tabular}[width=1\textwidth]{l|ccc}
\toprule[1.5pt]
\cmidrule(l){2-4} 
\multicolumn{1}{c}{Characteristics}  & \multicolumn{1}{|c}{\textbf{Train Set}}   & \textbf{Val Set}  & \textbf{Test Set}     
\\ \cmidrule(l){1-1} \cmidrule(l){2-4} 
\textbf{Age (years)} & &	&		\\
Range &18-93 &39-87	&19-85		\\
Average (Women) &42.6	&51.4	&37.5	\\
Average (Men) &57.4	&48.6	&62.5 	\\
\hline
\textbf{Cancer Subtype}(number) &- &-	&-\\	
Breast  	&23 	&8 	&3 \\
Lung 	&21	&11	&13\\
Prostate	&7	&2	&0\\
Colon	&15 	&3 	&3 \\
Renal cell carcinoma	&10 	&2 	&1 \\
Nasopharyngeal	&9	&3 	&1 \\
Others	&32 	&3 	&7 \\
\hline
\textbf{MESCC location} (number)&- &-	&-\\
Diffuse thoracic	&30 	&8 	&3  \\
C7-T2	&13 	&3 	&6 \\
T3-T10	&55 	&18 	&15\\
T11-L3	&31 	 &6 &8 \\
 \bottomrule[1.5pt]
\end{tabular}
\label{tab:dataset_1}
\end{table}
\noindent\textbf{Baselines.} To quantify the efficacy of the proposed framework, we use several baselines for performance comparison according to different aspects.

On the SSL aspect, we consider three SSL baselines:
\begin{itemize}
\item \textbf{P-Labeling}~\cite{lee2013pseudo}~\footnote{\url{https://github.com/iBelieveCJM/pseudo\_label-pytorch}} converts the model predictions to hard labels and then uses them to train against the task model.

\item \textbf{MixMatch}~\cite{berthelot2019mixmatch}~\footnote{\url{https://github.com/google-research/mixmatch}} mixes both labeled examples and unlabeled examples with label guesses and then makes use of consistency loss to improve the SSL model robustness.
\item \textbf{FixMatch}~\cite{berthelot2019mixmatch}~\footnote{\url{https://github.com/kekmodel/FixMatch-pytorch}} combines pseudo-labeling and consistency regularization simultaneously. It achieves SoTA results on CIFAR~\cite{krizhevsky2009learning} by combining these techniques with weak and strong data augmentations and using cross-entropy loss as the regularization criterion.
 \end{itemize}

On the AL aspect, we choose the following recent methods as baselines:
\begin{itemize}
\item   \textbf{R-Labeling}~\cite{figueroa2012active}~\footnote{\url{https://github.com/google/active-learning/tree/master/sampling\_methods}} uses random sampling that often serves as the lower bound of AL algorithms.
\item   \textbf{DBAL}~\cite{gal2017deep}~\footnote{\url{https://github.com/tanyinghui/DBALwithImgData}} takes advantage of recent advances in Bayesian deep learning  to choose the AL samples.
\item   \textbf{VAAL}~\cite{sinha2019variational}~\footnote{\url{https://github.com/sinhasam/vaal}} leverages the VAE-GAN structure to learn embedding in latent space and find out samples that are more likely to fall into the unlabeled pool.  

\item   \textbf{CSAL}~\cite{gao2020consistency} selects samples with the high inconsistency of predictions over a set of data augmentations. 

 \end{itemize}

\section{MESCC Dataset}\label{sec:MD}
\noindent\textbf{Background.} Spinal metastases are common and seen in up to 40\% of cancer patients~\cite{chiu2020spinal}. Up to 20\% of these patients develop complications including spinal cord compression which can lead to permanent neurological dysfunction if treatment is delayed. With the development of more effective systemic therapies (such as targeted and immunotherapy), the survival of patients with metastatic cancer has increased. Consequently, the incidence of spinal metastases is expected to rise~\cite{barzilai2018state}.

\begin{table}[t]
\caption{ \textbf{Two-grading statistics of the MESCC dataset.}}
\centering
\begin{tabular}[width=1\textwidth]{l|cc|c}
\toprule[1.5pt]
\multicolumn{1}{c|}{\multirow{2}{*}{Sets}} & \multicolumn{2}{c}{Two-grading}&\multicolumn{1}{|c}{\multirow{2}{*}{Total}}  \\  
\cmidrule(l){2-3} 
\multicolumn{1}{c|}{}  & \textbf{Low-grade}  & \textbf{High-grade}  &           
\\ \cmidrule(l){1-1} \cmidrule(l){2-4} 
Train &4,644 &563	&5,207	\\
Val &917 &94	&1,011	\\
Test &982&95	&1,077 \\
\hline
Total &6,543 &752	&7,295
\\ \bottomrule[1.5pt]
\end{tabular}
\label{tab:dataset_1}
\end{table}

\begin{table}[t]
\caption{ \textbf{Six-grading statistics of the MESCC dataset.}}
\centering
\begin{tabular}[width=1\textwidth]{l|cccccc|c}
\toprule[1.5pt]
\multicolumn{1}{c|}{\multirow{2}{*}{Sets}} & \multicolumn{6}{c|}{Six-grading} &\multicolumn{1}{c}{\multirow{2}{*}{Total}} \\       
\cmidrule(l){2-4} \cmidrule(l){5-7}
\multicolumn{1}{c|}{}  & \textbf{b0}  & \textbf{b1a}  & \textbf{b1b}     & \textbf{b1c}    & \textbf{b2}  & \textbf{b3}      &    \multicolumn{1}{c}{}
\\ \cmidrule(l){1-1} \cmidrule(l){2-4} \cmidrule(l){5-7}\cmidrule(l){8-8}
Train &3,752 &409	&483	&224	&136	&203&5,207\\
Val &756 &73	&88	&50	&23	&21&1,011\\
Test &849&82	&51 &	39	&30	&26&1,077\\
\hline
Total &5,357 &564	&622	&313	&189	&250&7,295
\\ \bottomrule[1.5pt]
\end{tabular}
\label{tab:dataset_2}
\end{table}

Suspicion for spinal metastases begins in the clinic, as $\geq$ 85\% patients present with back pain. Imaging is then required to confirm the presence of spinal metastases and the associated complications. MRI is the most accurate modality due to improved soft-tissue resolution, which allows assessment of the extent of metastatic bony involvement, compression fractures, and the presence of metastatic epidural spinal cord compression (MESCC)~\cite{di2020separation}. 

According to the above situation, we collected a metastatic epidural spinal cord compression (MESCC) dataset for method development and extensive evaluation, which aims to optimize MESCC diagnosis and classification for improved specialist referral and treatment.

\noindent\textbf{Data Collection.} Retrospective, manual extraction and anonymization of MRI spines from patients with known vertebral metastatic disease and thoracic MESCC was done over a ten-year period from September 2007 to September 2017 at two hospitals. Adult patients ($\geq$ 18 years) were included with selection of studies across different MRI scanners (GE and Siemens 1.5 and 3.0T platforms). MRI spines with instrumentation, suboptimal image quality (e.g., motion and cerebral spinal fluid flow artefacts) and non-thoracic spine regions were excluded. Axial T2-weighted DICOM images were utilized. Table 1 provides details on the MRI scanners and sequence parameters.

\begin{figure}[t]
\includegraphics[width=0.5\textwidth]{latex/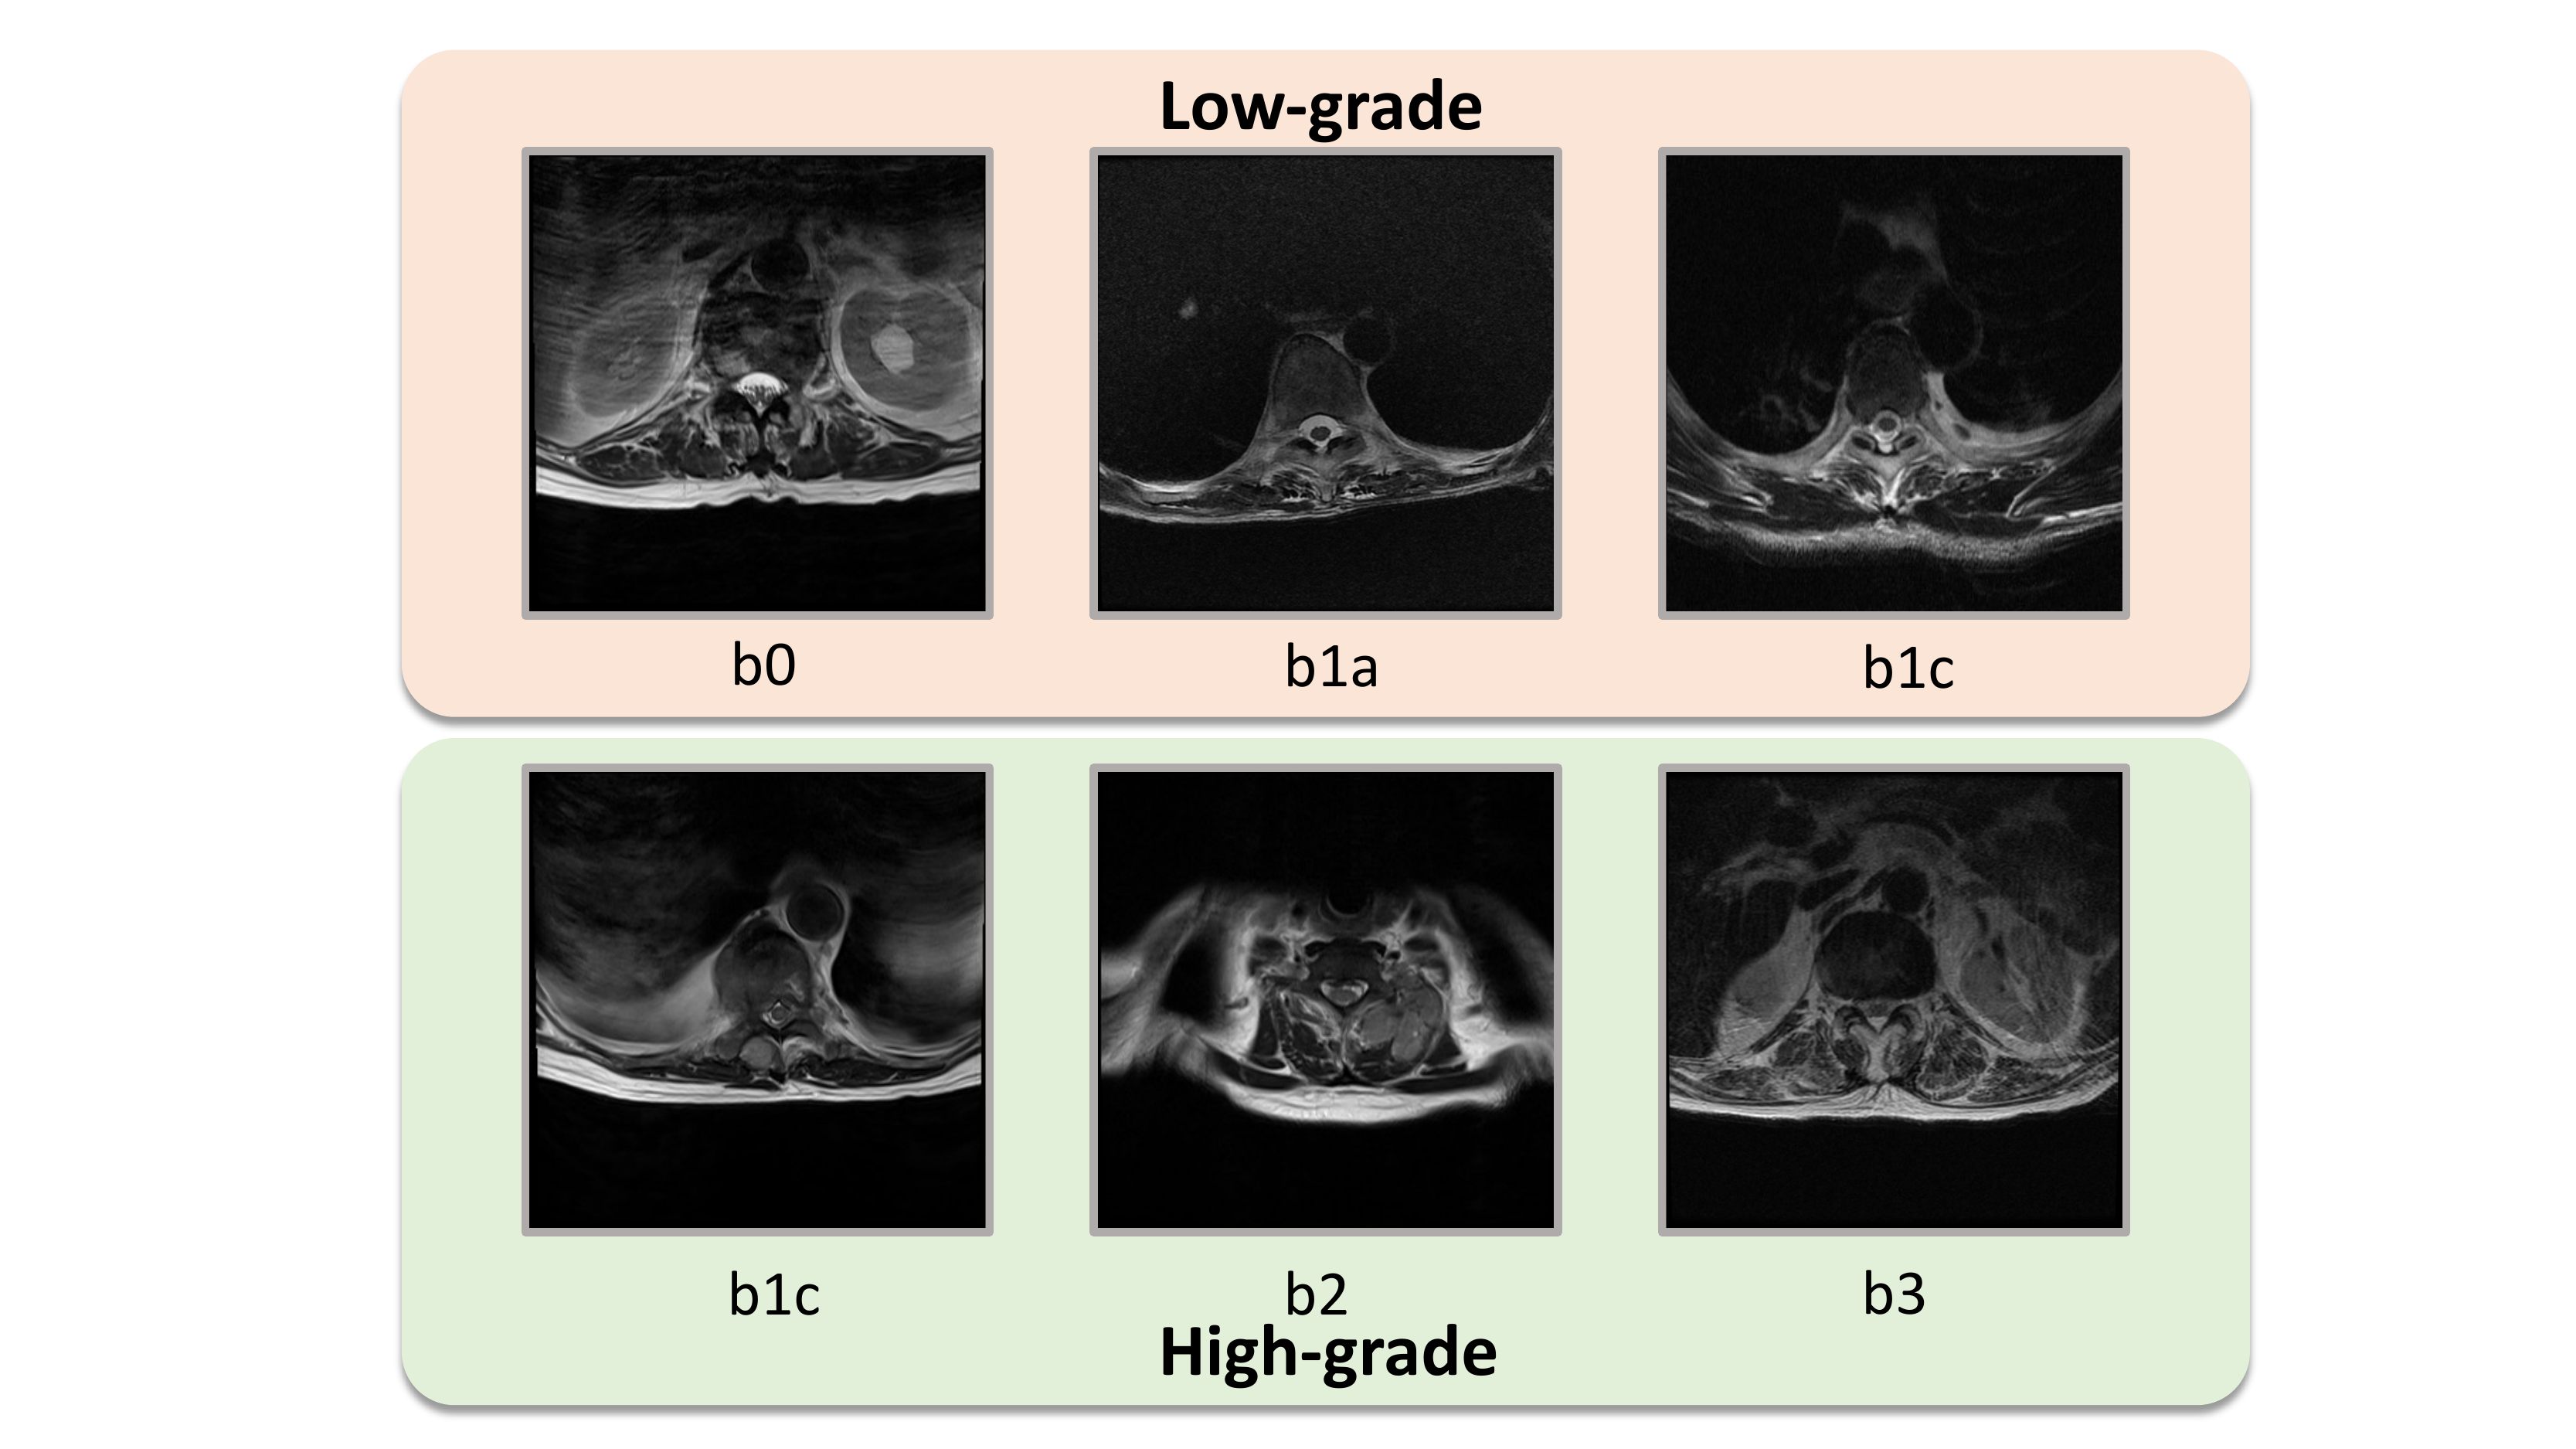}
\centering\caption{\textbf{Six grades (b0, b1a, b1b, b1c, b2, b3) and two grades (low-grade and high-grade)  of the MESCC   data.} }
\label{MESCC_sample}
\end{figure}

\begin{table}[t]
\small
\caption{ \textbf{Human evaluation of two-grading on MESCC dataset.}}
\centering
\begin{tabular}[width=1\textwidth]{l|ccc}
\toprule[1.5pt]
\cmidrule(l){2-4} 
\multicolumn{1}{c}{Reader}  & \multicolumn{1}{|c}{\textbf{Low-grade}}   & \textbf{High-grade}  & \textbf{Mean}     
\\ \cmidrule(l){1-1} \cmidrule(l){2-4} 
Neuroradiologist &95.01 &97.89	&95.26		\\
Radiation  Oncologist &96.03	&97.89	&96.19	\\
Spine Surgeon &97.04	&98.95	&97.21	\\

 \bottomrule[1.5pt]
\end{tabular}
\label{tab:human}
\end{table}

Internal training data were manually labeled by two board-certified radiologists with subspecialization in musculoskeletal radiology (10-years-experience) and neuroradiology (5-years-experience). Each radiologist labeled at least 100 MRI thoracic spine studies independently. Using an open-source annotation software~\footnote{\url{  https://github.com/tzutalin/labelImg}}, bounding boxes were drawn around the spinal canal to segment the region of interest (RoI) at the spinal canal along the thoracic spine (C7-T1 through to the conus at T12-L3).

The MESCC dataset consists of 7,295 medical images. When drawing each bounding box, the annotating radiologist employed the Bilsky classification~\cite{bilsky2010reliability} that consists of patients with six types of grades that are b0, b1a, b1b, b1c, b2, and b3. In general, we can also classify these grades into low-grade (i.e., b0, b1a, and b1b) and high-grade (i.e., b1c, b2, and b3) Bilsky MESCC (Figure~\ref{MESCC_sample}). Specifically, patients with low-grade are amenable to radiotherapy, while the patients with high-grade are more likely to require surgical decompression. Table~\ref{tab:dataset_1} and Table~\ref{tab:dataset_2} present the statistics of two-grading and six-grading on MESCC dataset. The dataset is randomly split into 70\% (5207) / 15\% (1011) / 15\% (1077) for the training/validation/test sets, respectively.

\noindent\textbf{Human Evaluation.}
     For better method development and extensive evaluation, we invited three experienced medical experts (Neuroradiologist, Radiation Oncologist, Spine Surgeon) to perform the human evaluation for the MESCC dataset. The details of the human evaluation are presented in Table~\ref{tab:human}.

\begin{figure}[t]
\includegraphics[width=0.53\textwidth]{latex/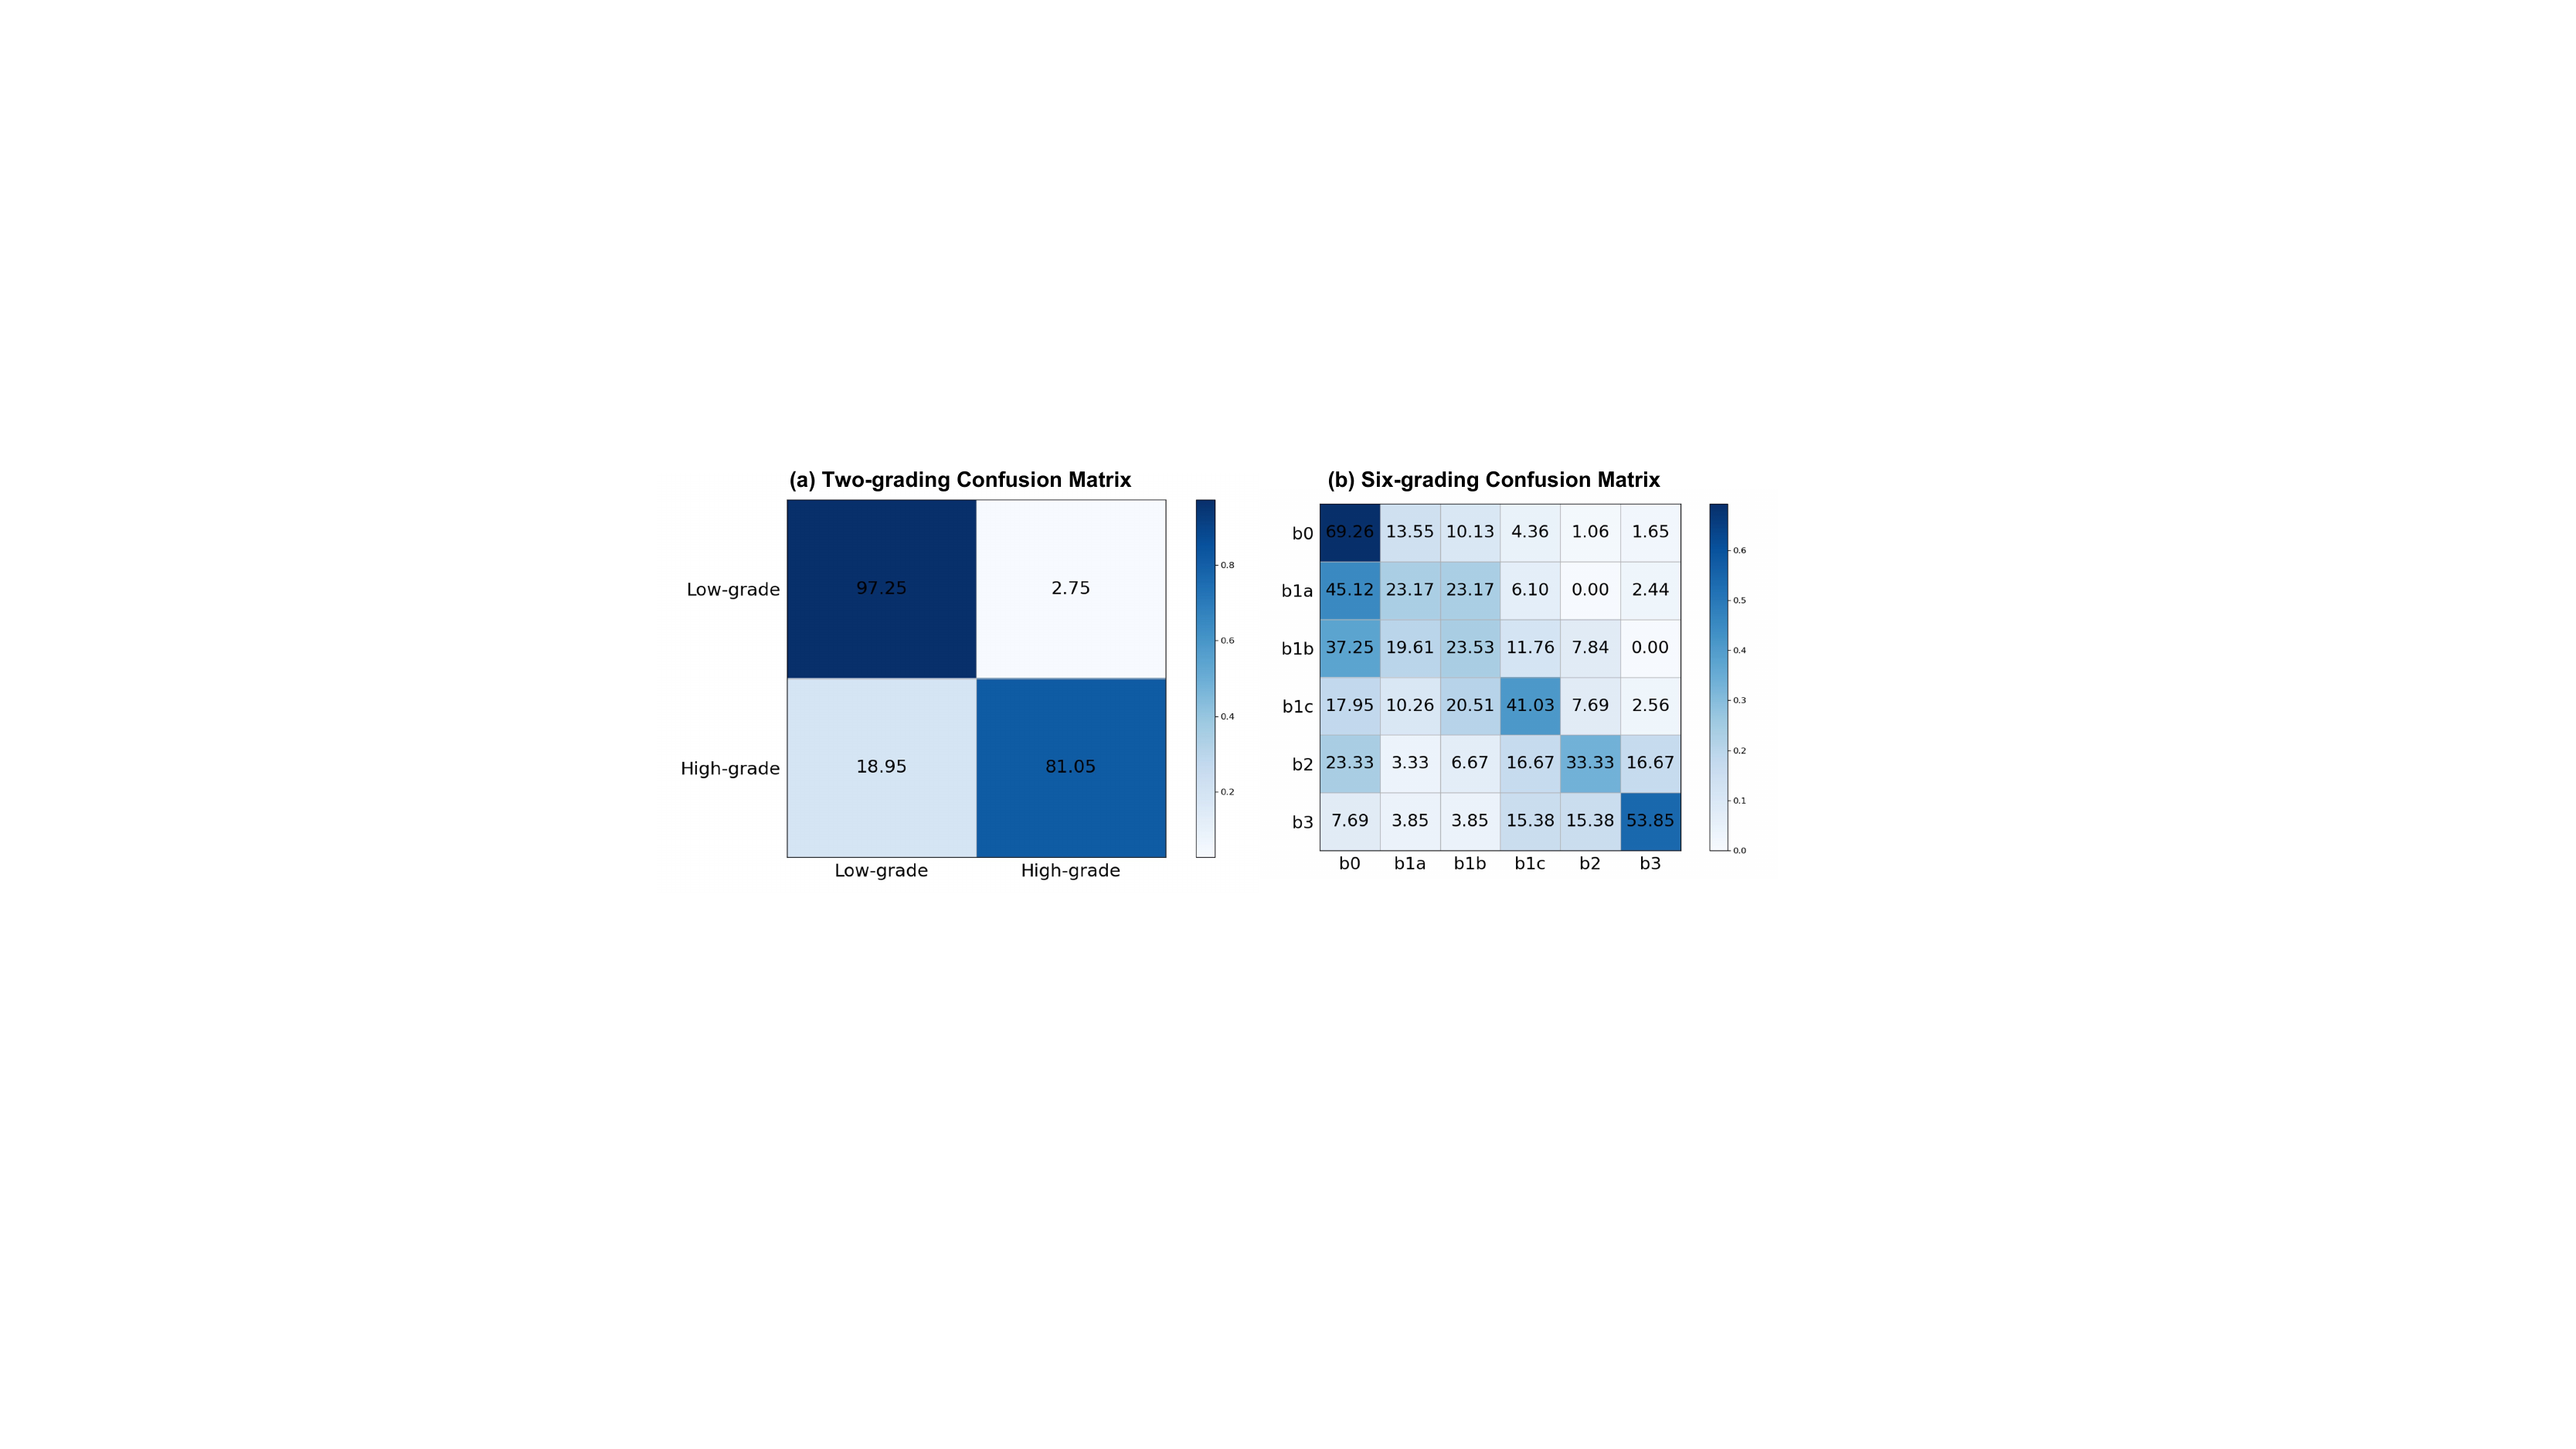}
\centering\caption{ \textbf{Confusion matrix of accuracy on MESCC dataset.} }
\label{confusion_matrix}
\end{figure}

\begin{table}[t]
\small
\caption{ \textbf{Performance comparison of different labeled setting on  MESCC dataset.}}
\centering
\begin{tabular}[width=1\textwidth]{l|cc}
\toprule[1.5pt]
\cmidrule(l){2-3} 
\multicolumn{1}{c}{Labeled Setting}  & \multicolumn{1}{|c}{\textbf{Two-grading}}   & \textbf{Six-grading}      
\\ \cmidrule(l){1-1} \cmidrule(l){2-3} 
30\% data (20\% AL selection) &95.82 &61.47		\\
50\% data (40\% AL selection) &97.49	&64.25		\\
75\% data (65\% AL selection) & \textbf{98.60}	&\textbf{66.67}		\\
 \cmidrule(l){1-1} \cmidrule(l){2-3}
100\% data (w/o AL selection)  &97.31	&65.00		\\
 \bottomrule[1.5pt]
\end{tabular}
\label{tab:diff_label}
\end{table}

 \begin{figure*}[t]
 \vspace{-0.4cm}
\includegraphics[width=1\textwidth]{latex/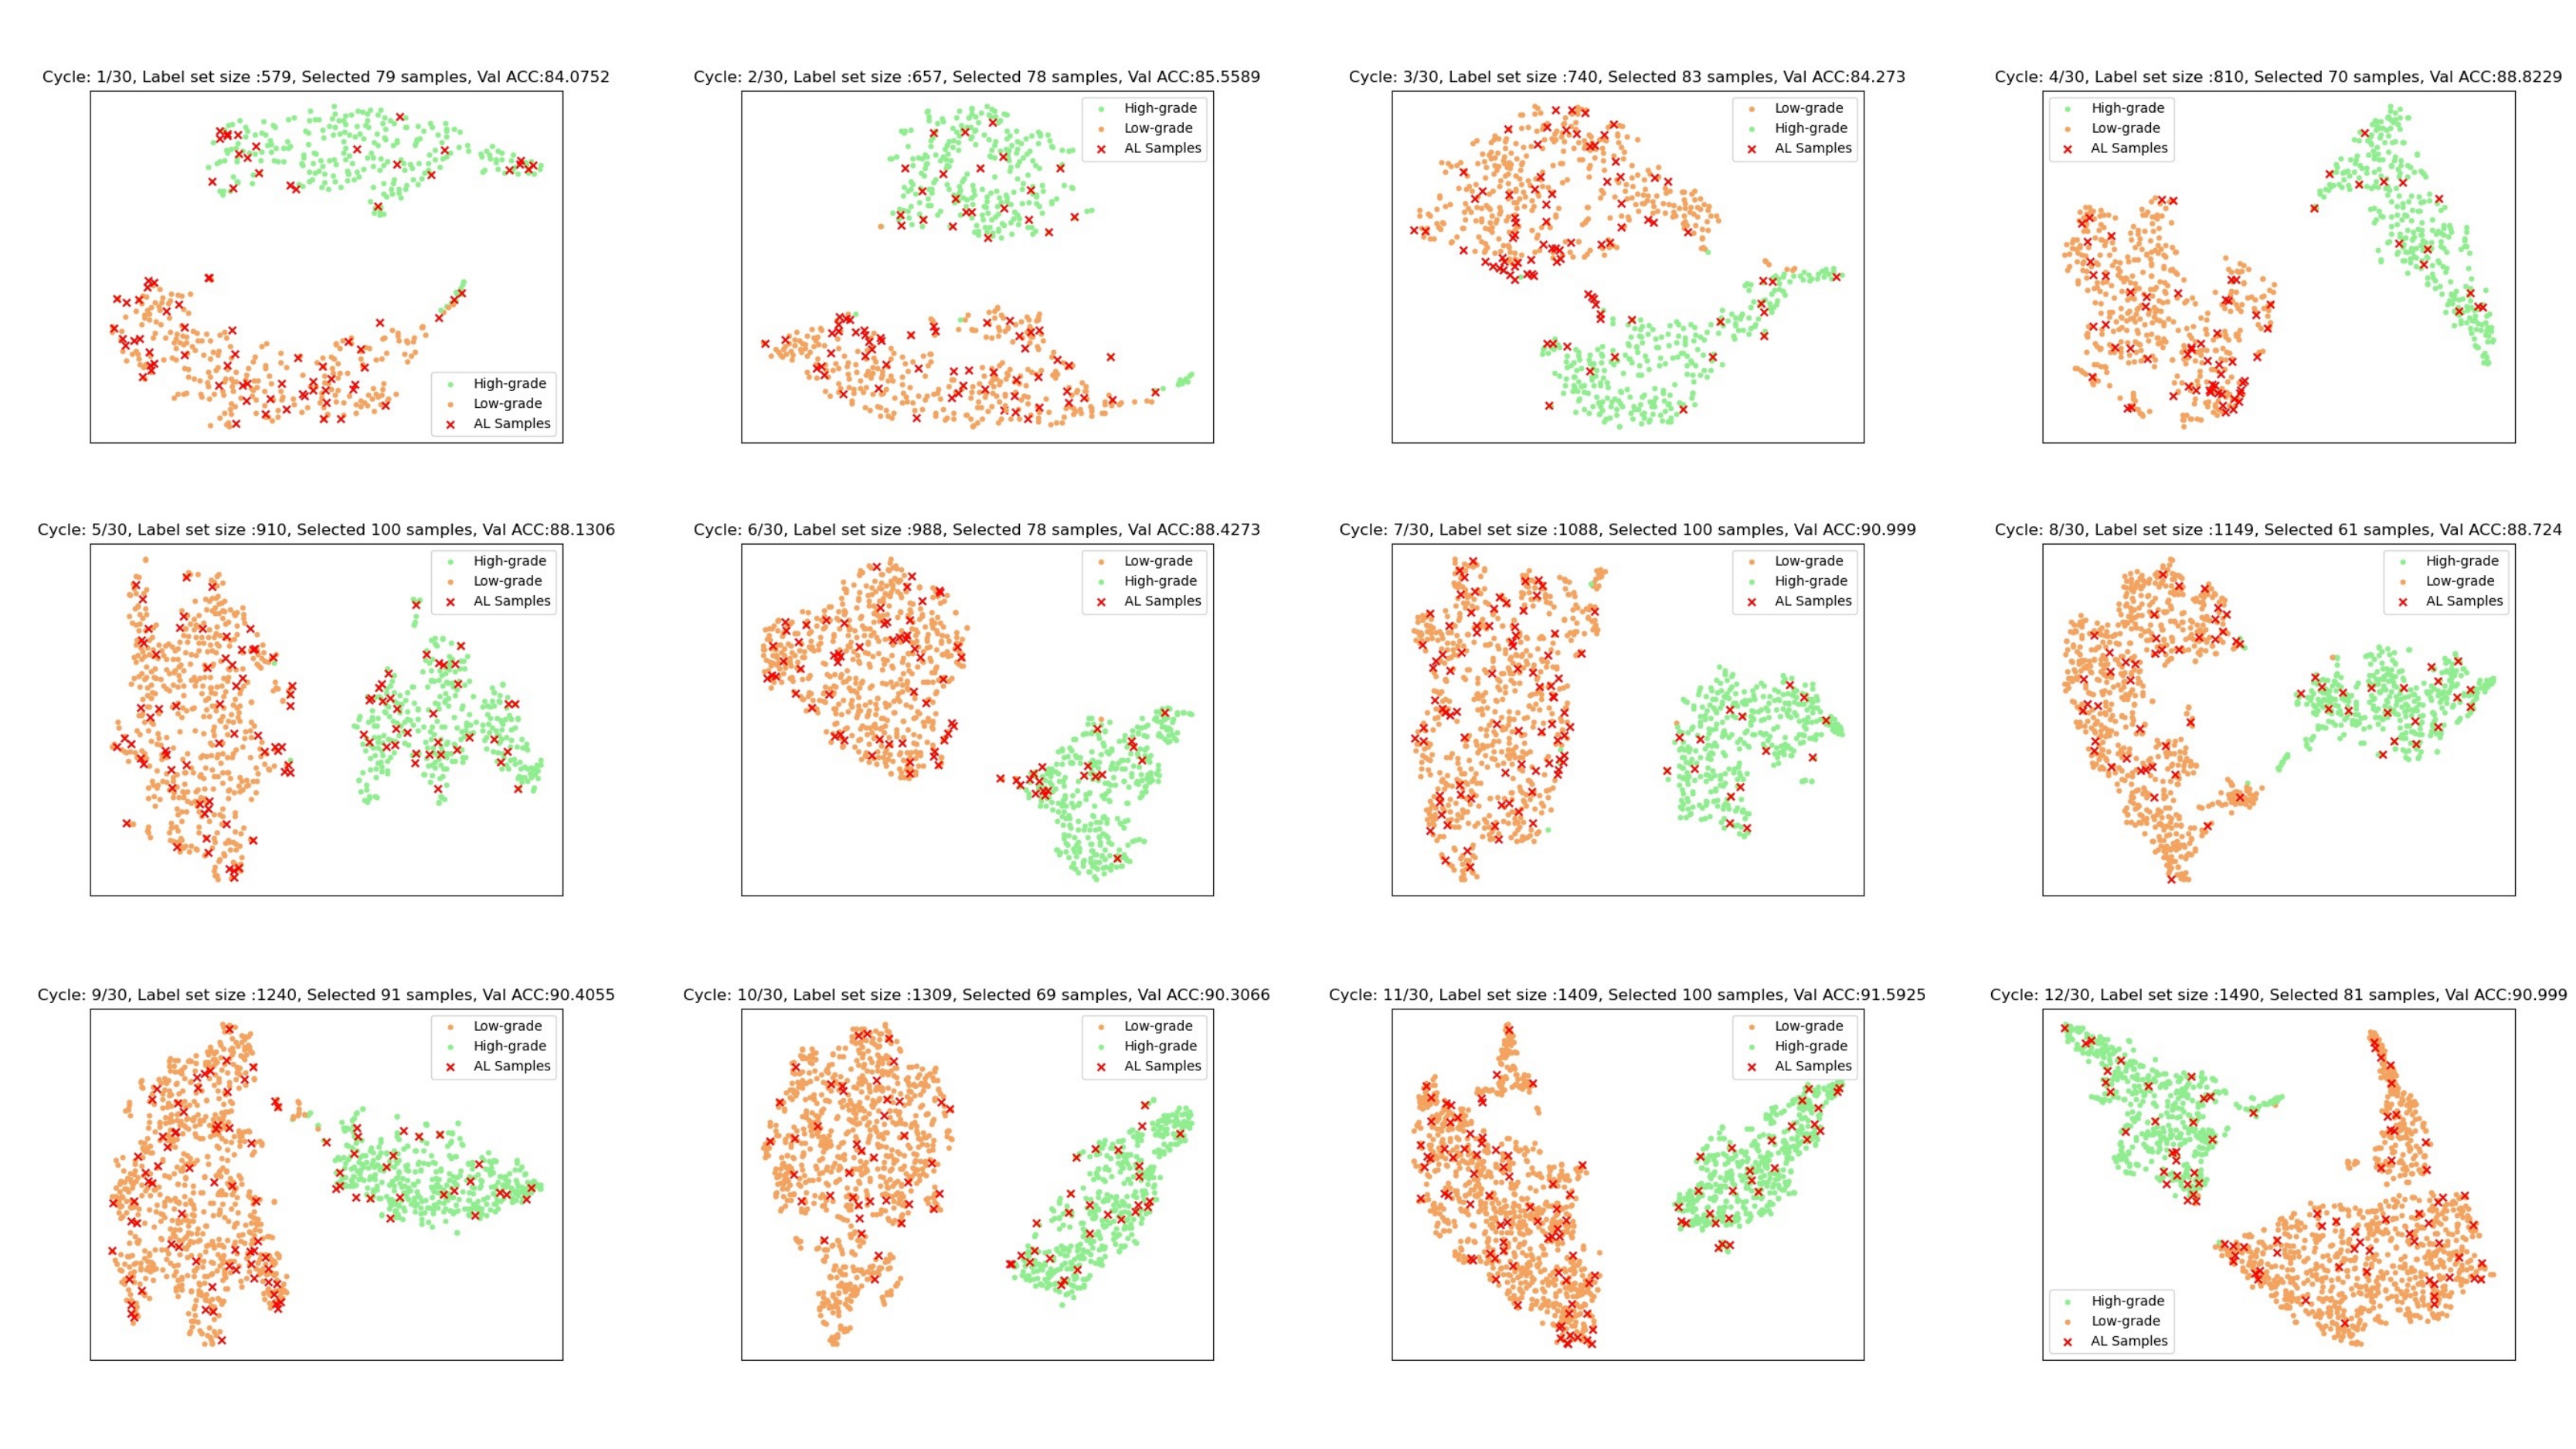}
\vspace{-0.6cm}
\caption{ \textbf{Visualization of Al selection behavior using tSNE embeddings in each training cycle.}  Orange and green dots represent the low-grade sample and high-grade sample in labeled pool, respectively. Red  marks indicate the annotation candidates.  }
\label{AL_selection}
\vspace{-0.2cm}
\end{figure*}

\vspace{-0.2cm}
 \begin{figure}[t]
 \centering
\includegraphics[width=0.4\textwidth]{latex/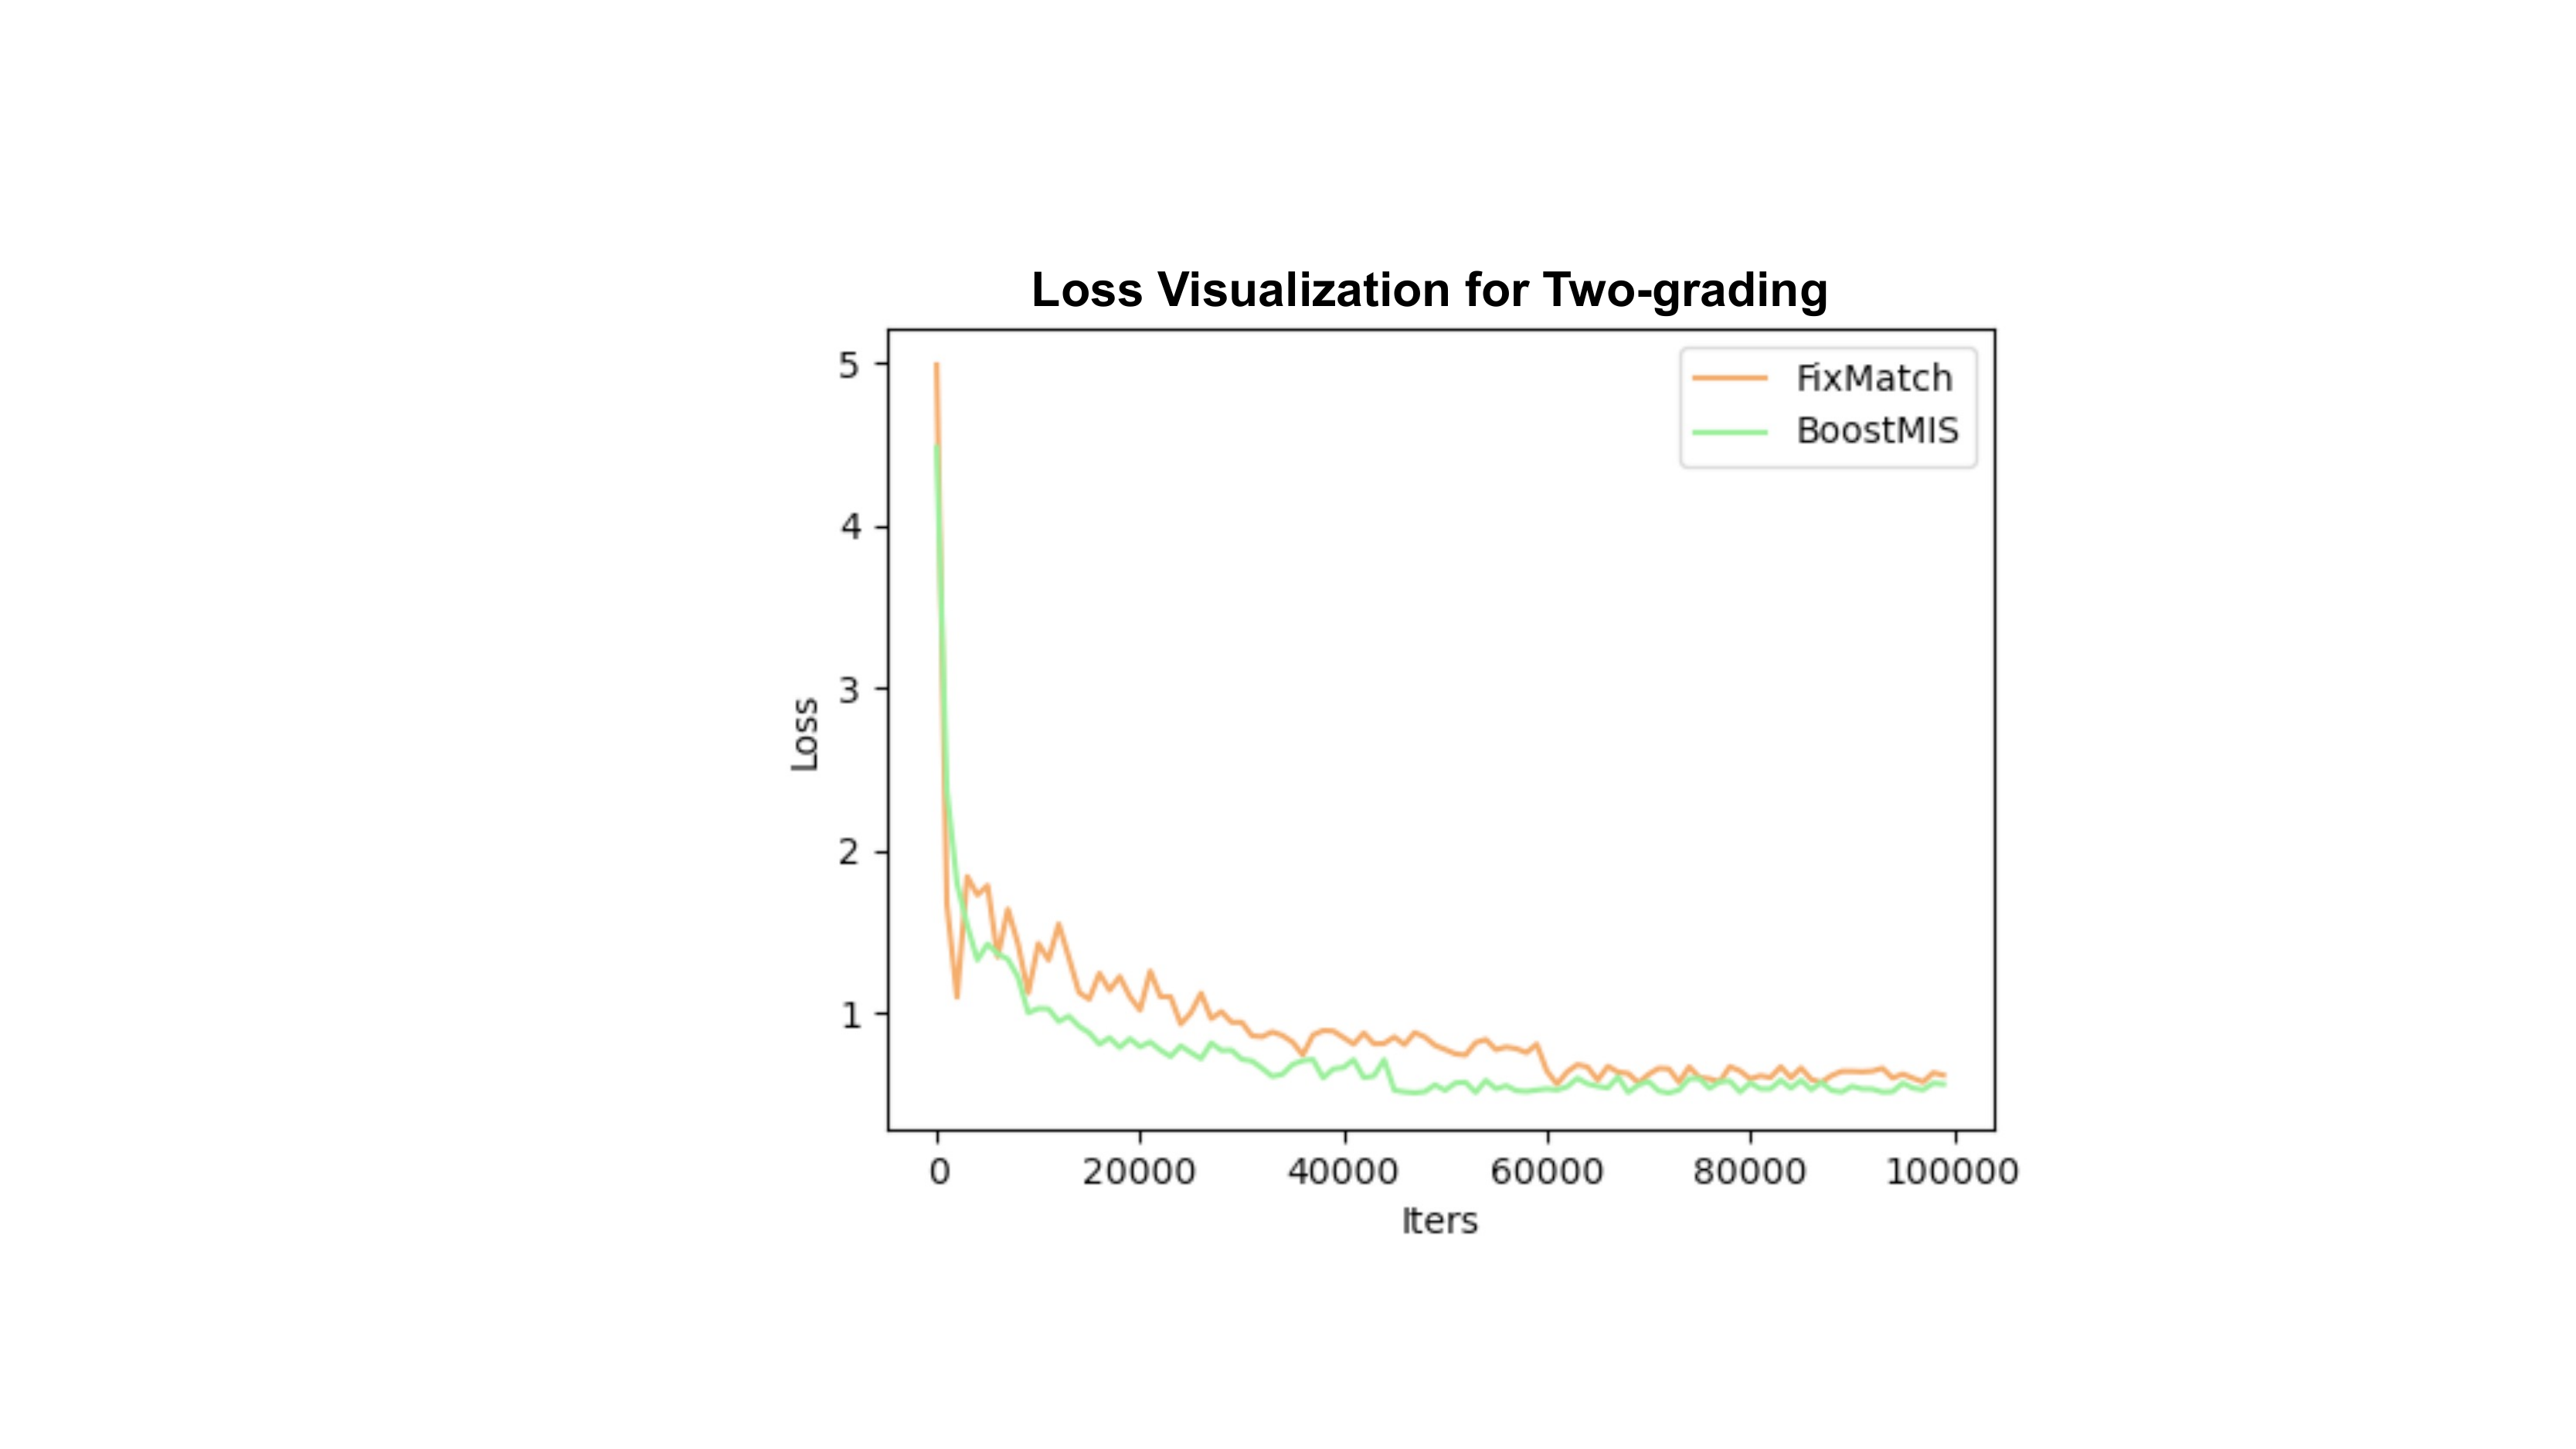}
\caption{  \textbf{Training loss for two-grading on MESCC dataset.} X-axis: iterative step; Yaxis: training loss. We depict the loss 
when the percentage of labeled pool reaches 30\%.}·
\label{loss}
\vspace{-0.2cm}
\end{figure}

\section{Experiments on MESCC dataset} \label{sec:exp_MESCC}
We conducted the additional experiments on the MESCC dataset to verify the strength of the proposed \method{}.

\noindent\textbf{Confusion Matrix.} The normalized confusion matrices of method for two-grading accuracy and six-grading accuracy are depicted in Figure~\ref{confusion_matrix}. From the results, we can observe that our method obtains a strong performance of two-grading. However, the six-grading results are not as strong as the two-grading. We speculate the main reasons are two folds: (1) (b0, b1a, b1b)/(b1c, b2, b3) samples have higher inter-class similarity in pixel-level, i.e., the model tends to classify similar medical images to wrong class (e.g., most of b1a samples classified to b0 and b1a). In fact, even human experts need to observe the details carefully to classify them correctly. (2) Except for b0, MRI images with other classes are insufficient. Due to insufficient data, the informative active annotation from our framework fails to obtain enough knowledge of the distribution of that data. It is difficult to construct the complex mapping of visual samples and their corresponding classes. Nevertheless, \method{} achieves the best performance compared to the state-of-the-art methods.

\noindent\textbf{Effect of Different Labeled Setting.}  Table~\ref{tab:diff_label} summarizes more results of the task model's performance under the different labeled settings. Using the entire datasets, the task model of Wide ResNet-50 can yield the accuracy of 97.31\% and 65.00\% for two-grading and six-grading, respectively. Most notably, our method outperforms the performance of fully supervised training only \textbf{\underline{75\% data (Row 3 VS Row 4)}}. \method{} that using 50\% samples yields a competitive result (Row 2 VS Row 4). It can be explained that our method can select the most informative samples, and these samples’ feature distribution benefits the task model’s training the most.

 \begin{table*}
\caption{\textbf{Performance comparison on COVIDx dataset.}  Superscript $^{\dagger}$ indicates that the model only employs the SSL algorithm.
AL$^{*}$ indicates that the SSL model (FixMatch) uses the corresponding AL annotation strategy. We report the accuracy of all these models when the percentage of labeled pool reaches 20\%/25\%/30\%. A larger score indicates better performance, and the top two scores of accuracy are in bold. Acronym notations of each model can be found in Section~\ref{sec:ID}.}
\centering
\begin{tabular}[width=1\textwidth]{l|c|ccc|ccc}
\toprule[1.5pt]
\multicolumn{1}{c|}{\multirow{2}{*}{\textbf{Methods}}} & \multicolumn{1}{c|}{\multirow{2}{*}{\textbf{AL$^{*}$}}} &\multicolumn{3}{c|}{COVIDx binary classification}                                                  & \multicolumn{3}{c}{COVIDx   three classification}

\\ \cmidrule(l){3-5} \cmidrule(l){6-8}
\multicolumn{1}{c|}{} &  & \textbf{20\% Labels}  & \textbf{25\% Labels}     & \textbf{30\% Labels}    & \textbf{20\% Labels}  & \textbf{25\% Labels}         & \textbf{30\% Labels}   \\ \cmidrule(l){3-5} \cmidrule(l){1-2} \cmidrule(l){6-8}
\textbf{P-Labeling}$^{\dagger}$~\cite{lee2013pseudo}                           &    & 73.15      &73.15   &75.70    &    75.60	& 77.82   & 78.63    \\     
\textbf{MixMatch}$^{\dagger}$~\cite{berthelot2019mixmatch}  
&   & 76.21     & 78.26    &80.05    &     80.04& 	81.85    & 83.26    \\  
\textbf{FixMatch}$^{\dagger}$~\cite{sohn2020fixmatch}                             
&   & 78.26      &80.31    &81.07   &     81.45&	83.47   &84.67       \\ 
 \midrule[1pt]
\textbf{R-Labeling}~\cite{figueroa2012active}  &  \checkmark                  
     &77.75     &79.80    &81.59      &     81.65& 	83.06   &84.47     \\    
\textbf{DBAL}~\cite{gal2017deep}    &    \checkmark                   
     &80.05     &82.86    &83.12  &     82.06&	83.87  &85.48    \\ 
\textbf{VAAL}~\cite{sinha2019variational} &  \checkmark                          
     &81.84     &\textbf{84.40}    &85.42     &    83.27 &	\textbf{85.28}   &86.09   \\
\textbf{CSAL}~\cite{gao2020consistency}&    \checkmark                         
     &\textbf{82.61}     &84.14    &\textbf{86.19}    &     \textbf{83.47}&	85.08  & \textbf{86.29}  \\ \midrule[1pt]
\textbf{\method{}}  &         \checkmark                  
     &\textbf{83.12}    &\textbf{85.68}   & \textbf{87.47}    &   \textbf{84.07}& 	\textbf{86.09}   & \textbf{88.10}\\
\bottomrule[1.5pt]
\end{tabular}
\label{tab:results_covidx}
\end{table*}

\begin{table}[t]
\small
\caption{ \textbf{Binary classification statistics of the COVIDx dataset.}}
\centering
\begin{tabular}[width=1\textwidth]{l|cc|c}
\toprule[1.5pt]
\multicolumn{1}{c|}{\multirow{2}{*}{Sets}} & \multicolumn{2}{c}{Binary classification}&\multicolumn{1}{|c}{\multirow{2}{*}{Total}}  \\  
\cmidrule(l){2-3} 
\multicolumn{1}{c|}{}  & \textbf{COVID-19 Negative}  & \textbf{COVID-19 Positive}  &           
\\ \cmidrule(l){1-1} \cmidrule(l){2-4} 
Train &15,068 &2,158	&17,226	\\
Test &100&291	&391 \\
\hline
Total &15,168 &2,449	&17717
\\ \bottomrule[1.5pt]
\end{tabular}
\label{tab:dataset_covid_1}
\end{table}

\noindent\textbf{Informative AL Selection in Each Cycle.} For a more intuitive view of how our model works for the informative active annotation, we visualize the AL selection in each training cycle. As shown in Figure~\ref{AL_selection}, we report the cycle number, size of the labeled pool, number of current AL selection and average two-grading accuracy on the validation set. This figure suggests that \method{} can evenly select the informative samples in each grade to balance the subsequent training in each training cycle. Evidently, the AL algorithm in \method{} can choose the unstable sample near the decision boundary and the uncertain sample that is representative in the data distribution space.These samples work together to offer useful information to the medical image SSL model, which improves performance.

\noindent\textbf{Convergence Analysis.}
To further verify the effectiveness of BoostMIS, we visualize the loss and corresponding iterative step in Figure~\ref{loss}. The loss of BoostMIS decreases faster and smoother than FixMatch, demonstrating its superior convergence speed. 
The major fluctuations of the loss in FixMatch may be due to the pre-defined threshold that lets pass most unlabeled data belonging to certain classes. \method{} uses the AL selection and adaptive threshold to accelerate convergence by leveraging informative samples with representative data distribution.

 \section{Experiments on COVIDx dataset}\label{sec:exp_COVID} 
 \noindent\textbf{COVIDx Dataset.}  To further evaluate
the effectiveness and generalisability  of proposed \method{},  
 we  introduce COVIDx dataset~\cite{wang2020covid}~\footnote{\url{https://github.com/lindawangg/}} and conduct extensive experiments on it.  COVIDx is an open access benchmark dataset  with the largest number of COVID-19 positive patient cases, and is the combination of five publicly available COVID-19 data repositories: 1) COVID-19 Image Data Collection~\cite{cohen2020covid}; (2) COVID-19 Chest X-ray Dataset Initiative~\footnote{\url{https://github.com/agchung/Figure1-COVID-chestxray-dataset}}; (3) Actualmed COVID19 Chest X-ray Dataset~\footnote{\url{https://github.com/agchung/Actualmed-COVID-chestxray-dataset}}; 4) COVID-19 radiography dataset~\footnote{\url{https://www.kaggle.com/tawsifurrahman/covid19-radiography-database}}; 5)
RSNA Pneumonia Detection Challenges dataset~\footnote{\url{https://www.kaggle.com/c/rsna-pneumonia-detection-challenge/data}}.
The task of Covid-19 diagnosis is image classification with three classes:  (i) \emph{Normal} (No infection), (ii) \emph{Pneumonia} (NonCOVID-19 infection, e.g., viral, bacterial, etc.), and (iii) \emph{COVID-19} (COVID-19 viral infection). COVIDx dataset also develops a binary classification (\emph{COVID-19 Negative} (Normal, Pneumonia) and \emph{COVID-19 Positive} (COVID-19). As these datasets are ever-updated during the ongoing pandemic, we specify the  statistics of the two classification tasks in Table~\ref{tab:dataset_covid_1} (binary classification) and  Table~\ref{tab:dataset_covid_2} (three classification).

 \begin{table}[t]
\small
\caption{ \textbf{Three classification statistics of the COVIDx dataset.}}
\vspace{-0.1cm}
\centering
\begin{tabular}[width=1\textwidth]{l|ccc|c}
\toprule[1.5pt]
\multicolumn{1}{c|}{\multirow{2}{*}{Sets}} & \multicolumn{3}{c}{Three classification}&\multicolumn{1}{|c}{\multirow{2}{*}{Total}}  \\  
\cmidrule(l){2-4} 
\multicolumn{1}{c|}{}  & \textbf{Normal} & \textbf{Pneumonia}  & \textbf{COVID-19}  &           
\\ \cmidrule(l){1-1} \cmidrule(l){2-5} 
Train &8,751 &5,964&2,158	&16,873	\\
Test &100&105&291	&496 \\
\hline
Total &8,851 &6,069&2,449	&17,369
\\ \bottomrule[1.5pt]
\end{tabular}
\label{tab:dataset_covid_2}
\end{table}

\noindent\textbf{Experimental Results on COVIDx Dataset.} We compare the performance of our approach to the SSL and AL state-of-the-art methods of image classification task and summarize the results
in Table~\ref{tab:results_covidx}. As for the global testing accuracy, we can see that our method significantly outperforms the baselines, and the superiority is consistently observed on all labeled settings (From 20\% samples to 30\% samples). The overall results of all methods on the COVIDx dataset are similar to the MESCC dataset, the AL-based SSL models achieve a better accuracy according to pure SSL methods. This proves again that the appropriate strategy of AL selection can bring valuable samples (e.g., representative local data distribution) to improve the SSL model's performance. It is worth noting that our \method{} outperforms SSL baseline FixMatch with the same amount of labeled data by a large margin (e.g., \textbf{\underline{6.4\% improvement with 30\% labeled samples}}). Our framework also brings a huge reduction of annotation cost to reach a higher performance (\method{} with 20\% data: 84.14\%, FixMatch with 30\% data: 81.07\%). In other words, the strong results on the COVIDx dataset indicate the effectiveness of the proposed \method{} again.

\begin{table}
\small
\caption{Experimental results of Macro Precision (MP), Macro F1 score (MF1), Macro Recall (MRC) on COVIDx dataset.}
\centering
\setlength{\tabcolsep}{1.4mm}{
\begin{tabular}[width=1\textwidth]{l|cccccc}
\toprule[1.5pt]

\multicolumn{1}{c|}{\multirow{2}{*}{\textbf{Methods}}} & \multicolumn{3}{c}{Binary classification}                                                  & \multicolumn{3}{c}{Three classification}\\

\cmidrule(l){2-4}\cmidrule(l){5-7}
\multicolumn{1}{c|}{}  & \textbf{MP}  & \textbf{MF1}  & \textbf{MRC}     & \textbf{MP}    & \textbf{F1}  & \textbf{MRC}     
\\ \cmidrule(l){1-4}\cmidrule(l){5-7} \textbf{P-Labeling}~\cite{lee2013pseudo}  
                                                   &73.40&73.36	&80.40	&74.8 &81.41 &76.54	\\
\textbf{MixMatch}~\cite{berthelot2019mixmatch}   &77.89&78.16	&86.27	&79.82&81.83	&86.76\\
\textbf{Fixmatch}~\cite{sohn2020fixmatch}  &78.55&79.14	&86.96	&81.13& 87.98	&83.30	\\
\hline
\textbf{R-Labeling}~\cite{figueroa2012active}    &78.55&79.49	&86.64	&80.88&83.11	&87.85	\\
\textbf{DBAL}~\cite{gal2017deep}  &79.96&	81.13	&88.33&81.92	&84.14&88.66	\\
\textbf{VAAL}~\cite{sinha2019variational}    &81.72&83.42	&89.88	&82.30 &88.33 &84.42	\\
\textbf{CSAL}~\cite{gao2020consistency}  &\textbf{82.36}&\textbf{84.19}	&\textbf{90.39}	&\textbf{82.58} &\textbf{88.46} &\textbf{84.61}	\\
\bottomrule[1.5pt]
\textbf{\method{}}  &\textbf{83.47} &\textbf{85.50}	&\textbf{91.25}	&\textbf{84.53} &\textbf{90.32} &\textbf{86.71}
\\ \bottomrule[1.5pt]
\end{tabular}}
\label{tab:result_1}
\end{table}

To make the experimental results more comprehensive, we also explored the sensitivity of the models to each class. By presenting the confusion matrices for the models shown in Figure~\ref{confusion_matrix_covid}, we further demonstrate that our \method{} can obtain a high class-wise accuracy for each class of samples. In particular, our approach effectively classifies almost all COVID-19 Negative (99.00\%) and Normal (95.00\%) samples. The classification results of COVID-19 also present relatively strong results (83.51\% and 84.54\%). In contrast to the relatively poor performance of six-grading in the MESCC dataset, we can observe that our model achieves consistent superiority for the binary and three classification tasks. Our intuition is that the annotations for each class in the COVIDx dataset are sufficient to train our \method{}. The SSL model can benefit from the informative samples taken from the adversarial unstability selector and balanced uncertainty selector to obtain higher performance.

As shown in Table~\ref{tab:result_1}, the performance increases consistently on other metrics as well. Overall, compared to state-of-the-art SSL model FixMatch, our \method{} make a considerable gain on Macro Precision (4.92\% and 3.40\%), Macro F1 score ( 6.36\% and 2.34\%) and Macro Recall (4.29\% and 3.41\%) for binary and three classification, respectively. Moreover, our \method{} also outperforms the state-of-the-art AL model CSAL on all the metrics.

In summary, we propose adaptive pseudo-labeling and informative active annotation that leverage the unlabeled medical images and generate a mutually collaborative learning paradigm
 to improve the performance of the medical image SSL model. Extensive experimental studies of \method{} on MESCC and COVIDx datasets verify 
its effectiveness and generalizability for medical image classification tasks with a limited annotation cost.

\begin{figure}[t]
\includegraphics[width=0.51\textwidth]{latex/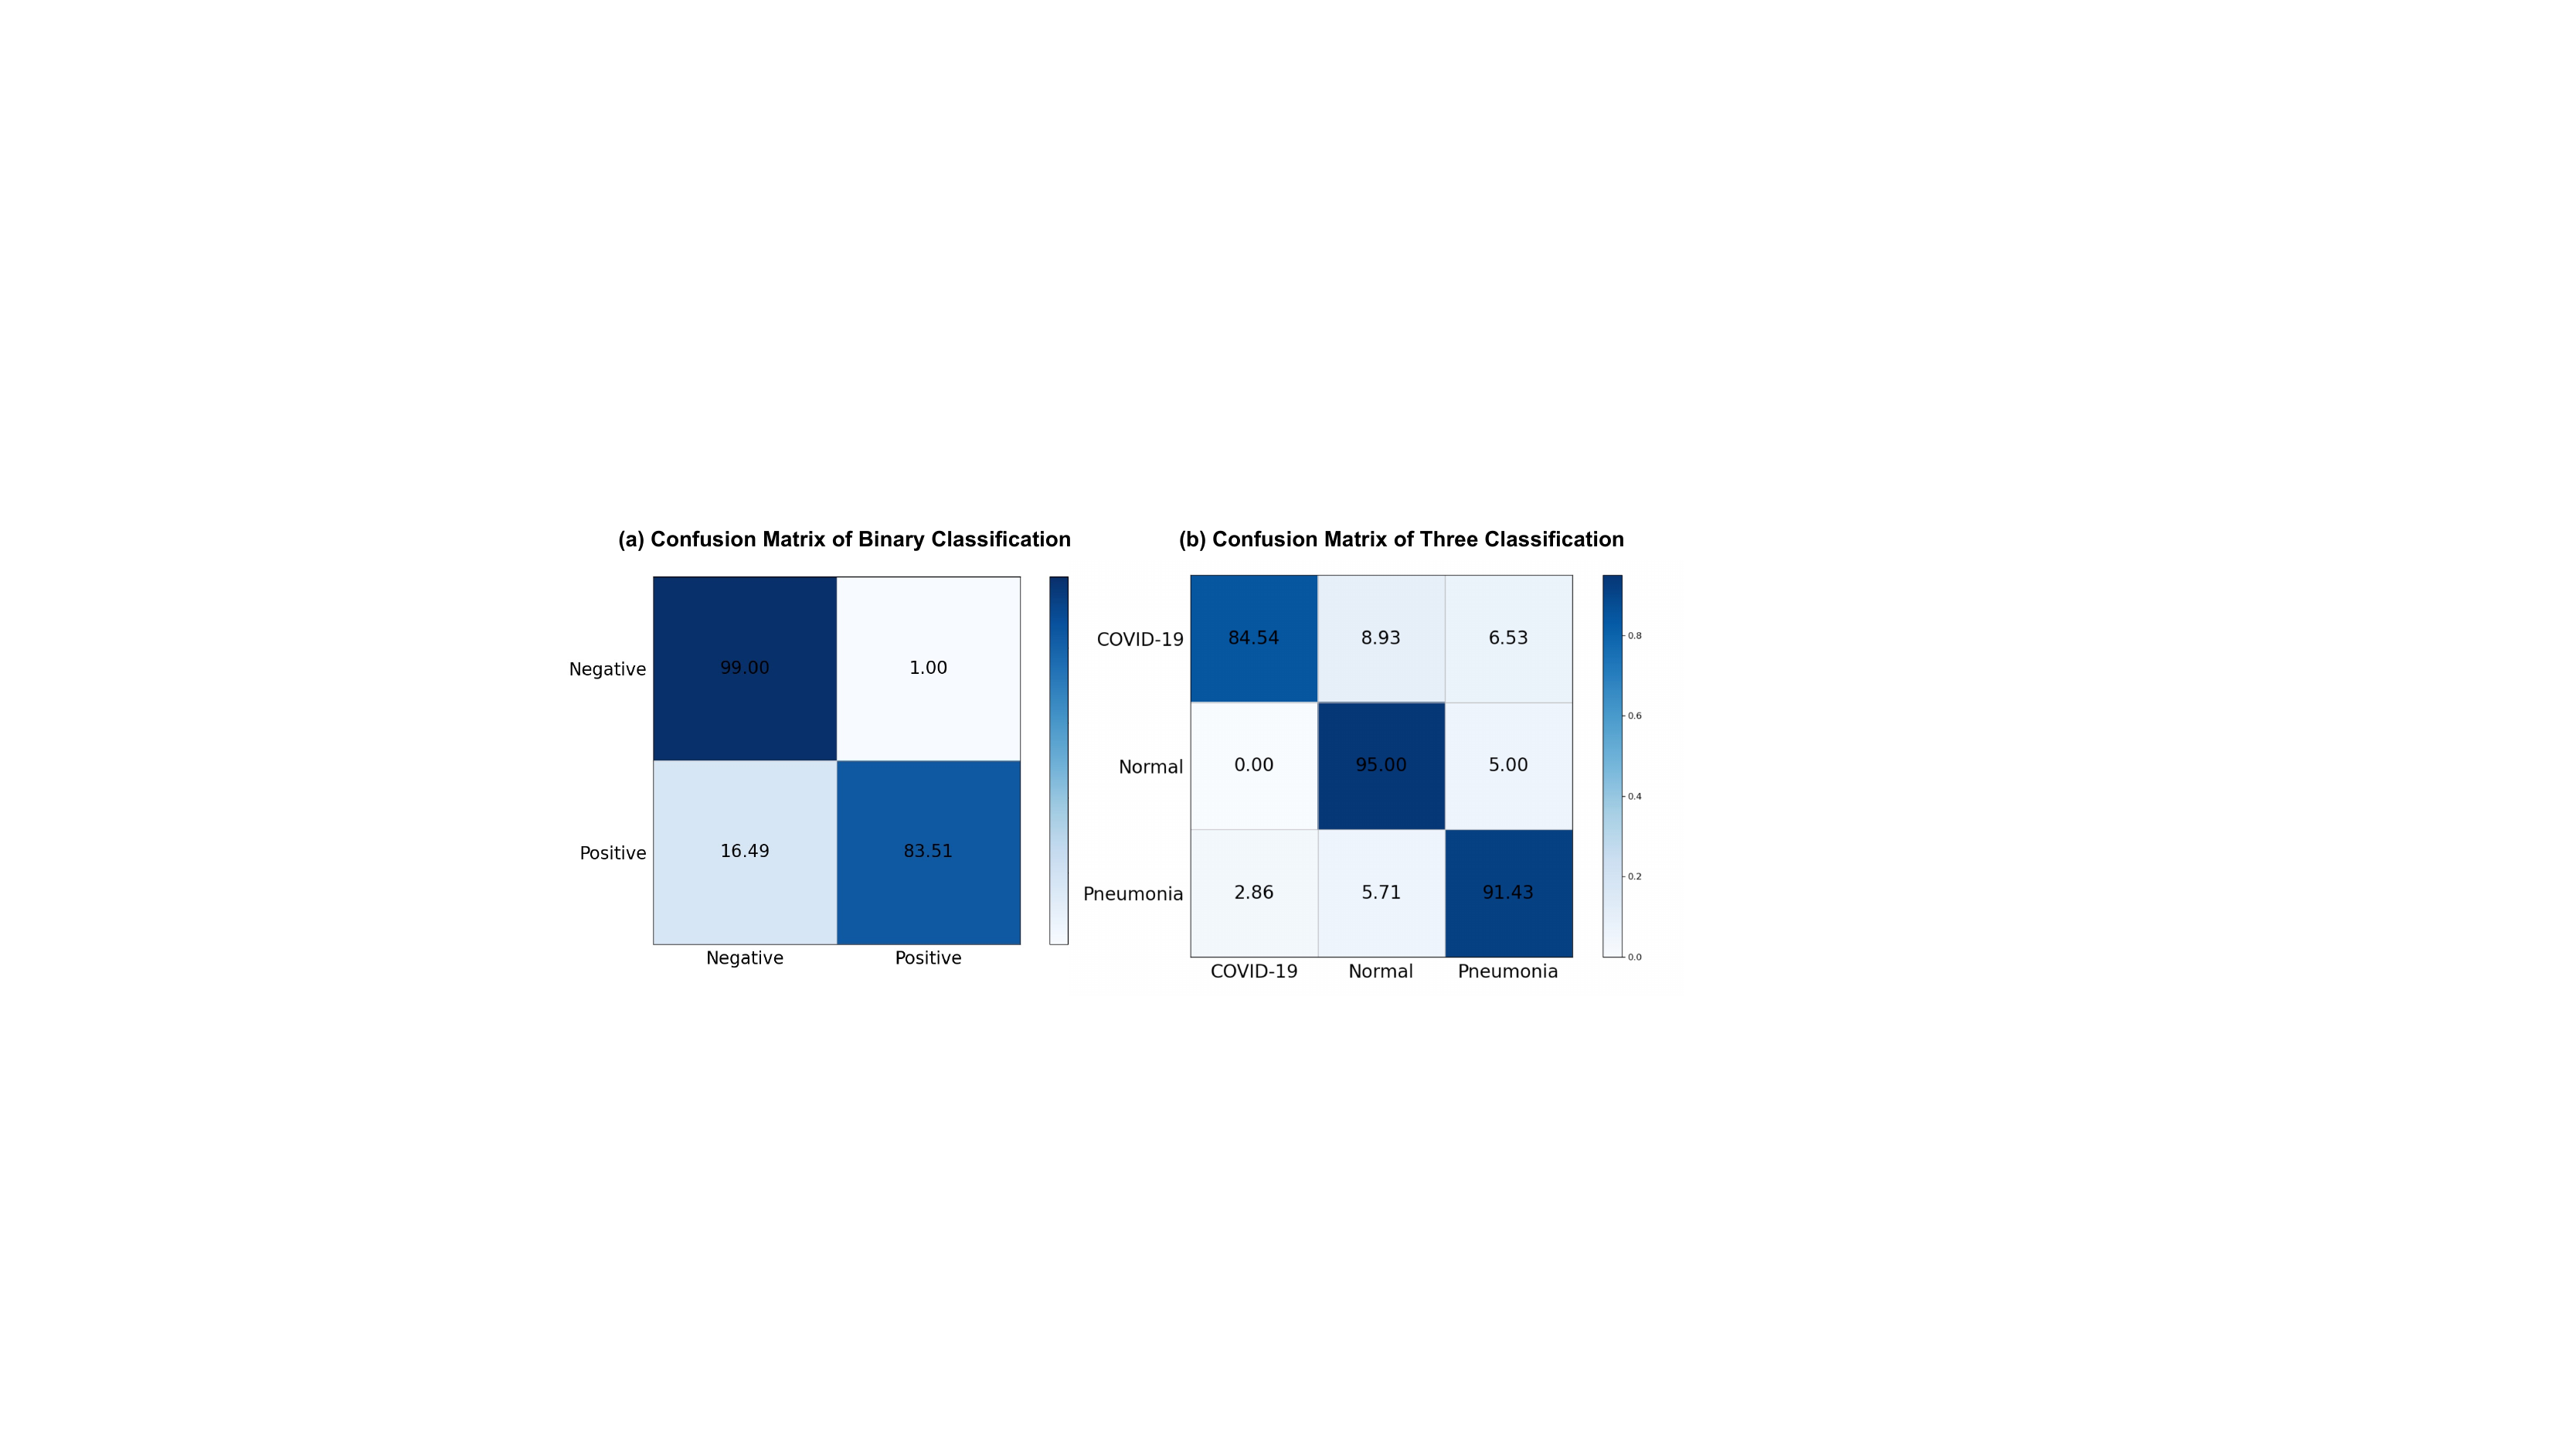}
\centering\caption{ \textbf{Confusion matrix of accuracy on COVIDx dataset.} }
\label{confusion_matrix_covid}
\end{figure}

\begin{table}[t]
\caption{ \textbf{Comparison of training duration. }}
\centering
\begin{tabular}[width=1\textwidth]{l|c}
\toprule[1.5pt]
\cmidrule(l){2-2} 
\multicolumn{1}{c}{Methods}  & \multicolumn{1}{|c}{\textbf{Training time}}      
\\ \cmidrule(l){1-1} \cmidrule(l){2-2} 
FixMatch &6 hours 	\\
Adaptive Pseudo Labeling &4 hours			\\
\method{} & \textbf{4 hours per AL cycle}			\\
 \bottomrule[1.5pt]
\end{tabular}
\label{tab:time}
\end{table}

\section{Limitations and Societal Impact}\label{sec:LSI}
\noindent\textbf{Limitations.} In terms of training time, Table~\ref{tab:time} illustrates that the SSL model in \method{} leads to an improvement in convergence speed according to FixMatch. However, \method{} requires multiple rounds of AL sampling and SSL training, i.e., the training duration is much longer than a pure SSL model. For instance, if the AL budget has a capacity of 20\% data and AL samples 5\% annotation candidates in each cycle, BoostMIS needs 4 AL cycles to train the SSL model with 16 hours of training time. Certainly, we can increase the number of AL selections in each cycle and expand the size of the initial labeled pool. It also boosts the SSL model's performance with shorter training time.

\noindent\textbf{Societal Impact.} This work involves some privacy concerns. For example, the proposed MESCC dataset is made up of MRI scans of adult patients. We will, however, provide the MESCC dataset's medical image features that safeguard patients' privacy and contribute to the AI MESCC diagnosis community.

% \begin{figure*}[t]
% \includegraphics[width=1\textwidth]{latex/pic/step_samples.pdf}
% \label{AL_selection}
% \centering\caption{ Al selected samples in each training cycle. }
% \end{figure*}
